# Supplementary material for: Efficient and Near-Optimal Smoothed Online Learning for Generalized Linear Functions
Source: arXiv:2205.13056 source file (2022-05-25)
Supplement: Supplementary file 1 [file mistake_app.tex]

%!TEX root = ../neurips_submission.tex

\section{Max Margin Classification with adversarial contamination.}
\ac{Fix contamination model to account for changing labels in the history.}
Suppose we are now in the smoothed online classification setting with noise.  In other words, suppose that at each time step $t$, we sample $x_t \sim p_t$ where $p_t$ is $\sigma$-smooth with respect to $\mu$ and then we predict $\yhat_t$.  Then we suffer a mistake if $\yhat_t \neq y_t$.  We observe, however, only $\widetilde{y}_t$, where we know that $\widetilde{y}_t = \yhat_t$ for all but $\alpha$ many time steps.  Suppose that the $(x_t, y_t)$ are indeed linearly separable.  For any vector $w$, let
\begin{align}
    U_{t,\alpha}(w) = \left\{ s < t | y_s \inprod{w}{x_s} > \left(\abs{\inprod{w}{x}}\right)_{(\alpha)} \text{ and } y_s = 1\right\} \cup \left\{ s < t | y_s \inprod{w}{x_s} > \left(\abs{\inprod{w}{x}}\right)_{(\alpha)} \text{ and } y_s = -1\right\}
\end{align}
i.e., we remove the points $(x_s, y_s)$ that have the $\alpha$-smallest margin with respect to $w$ in each cluster.  Now, we let
\begin{align}
    w_t = \argmax_{\substack{w \in \rr^d \\ y_s \inprod{w}{x_s} \geq 1 \text{ for all } s \in U_{2\alpha}(w)}} \norm{w}
\end{align}
be the robustified max-margin estimator.  In words, $w_t$ is the linear separator that maximizes the margin between those $x_s$ labelled $1$ and those labelled $-1$, ignoring the $\alpha$ points closest to the decision boundary in each cluster.  We then predict $\yhat_t = \sign(\inprod{w_t}{x_t})$.  We have the following result:
\begin{proposition}\label{prop:maxmarginnoisy}
    Suppose we are in the above situation and we use the robustified max-margin strategy.  Suppose further there is some $w^\ast$ such that $y_t \inprod{w^\ast}{x_t} \geq 1$ for all $t$.  Then, with probability at least $1 - \delta$,
    \begin{equation}
        \reg_T \leq 10 (2 \alpha + 1) \log\left(\frac{2 \Delta_0 T}{\sigma \delta}\right)
    \end{equation}
    In particular,
    \begin{equation}
        \ee\left[\reg_T\right] \lesssim \alpha \log\left(\frac{\Delta_0 T}{\sigma}\right)
    \end{equation}
\end{proposition}
\begin{proof}
    We first claim that with the proposed algorithm, we can make at most $2 \alpha + 1$ mistakes before the size of the margin shrinks by a factor of 2.  Indeed, note that after we have made $2 \alpha + 1$ mistakes, pigeonhole ensures that one of the clusters has at least $\alpha + 1$ mistakes, which in turn implies that $w_t$ can is updated so that the $x_s$ with minimal $\abs{\inprod{w_t}{x_s}}$ is now correctly classified.  In so doing, the margin shrinks by a factor of $2$.  We now present an argument similar to that of Proposition \ref*{prop:logarithmicrate}.

    Fix a set of positive integers $h_k$ for $k \in \mathbb{N}$.  Let $\tau_0 = 0$ and for all $m > 0$, let
    \begin{align}
        \tau_m = \tau_{m-1} + \inf\left\{k > 0 \bigg| \sum_{j = 1}^k \mathbb{I}[\yhat_s \neq y_s \text{ for } \tau_{m-1} + (j-1) h_m \leq s \leq \tau_{m-1} + j h_m] > 2 \alpha\right\}
    \end{align}
    Furthermore, let $T(m) = \sum_{k = 1}^m (\tau_k - \tau_{k-1}) h_k$ and
    \begin{equation}
        t_m^j = \inf\left\{t > T(m-1) \bigg| \sum_{t = \tau_{m-1}}^{t} \mathbb{I}[\yhat_t \neq y)t] > j  \right\}
    \end{equation}
    In words we consider epochs of length $h_m$, whose length can change every time we make $2 \alpha$ mistakes in an epoch.  We have $T(m)$ the time of the $m^{th}$ change of epoch and $\tau_m$ the number of epochs of length $h_m$ we have to go before we make $2\alpha$ mistakes; we also have $t_m^j$ is the time of the $j^{th}$ mistake in a unique epoch after the $m^{th}$ change of epoch size.  Let
    \begin{equation}
        A_m = \sum_{k = 1}^m \sum_{\substack{T(m-1) \leq s \leq T(m) - 1 \\ s \neq t_m^j}}\mathbb{I}[\yhat_s \neq y_s]
    \end{equation}
    be the number of ``repeat mistakes,'' i.e., the number of mistakes we make in an epoch that is not the first mistake.  Let $\pi_m = \min\left(\frac{\Delta_m}{\sigma}, 1\right)$, where $\Delta_m$ is an upper bound on the $\mu$-measure of the margin.  Then, just as in \eqref{eq:extramistakes}, we have that with probability at least $1 - \delta$, for all $m$ it holds that:
    \begin{equation}
        A_m \leq \log\left(\frac 1\delta\right) + (e - 1) \sum_{k = 1}^m \pi_k (\tau_k - \tau_{k-1}) (h_k - 1)
    \end{equation}
    which follows by the same Ville's inequality-based argument as before.  By a union bound, we may apply \eqref{eq:tauseparation} to get that with probability at least $1 - \delta$, it holds for all $m$ that
    \begin{equation}
        (\tau_m - \tau_{m-1}) \geq \max\left(2 \alpha + 1, (2 \alpha + 1)\log\left(\frac{\delta}{\pi_m h_m (2 \alpha + 1)}\right)\right)
    \end{equation}
    Now we note that
    \begin{equation}
        T \geq T(m) = \sum_{k = 1}^m (\tau_k - \tau_{k-1}) h_k
    \end{equation}
    and, further, that if $m_T$ is the maximal $m$ such that the preceding displa holds,
    \begin{equation}
        \reg_T \leq (2 \alpha + 1)m_T + A_{m_T}
    \end{equation}
    Thus, using the fact that $\pi_k \leq 2^{-k} \Delta_0 / \sigma$, we have that with probability at least $1 - 2\delta$,
    \begin{align}
        T &\geq (2 \alpha + 1) \sum_{k = 1}^{m_T} \log\left(\frac{ 2^k \sigma \delta}{\Delta_0 h_k T}\right) h_k \\
        \reg_T &\leq (2 \alpha + 1)\left(m_T + \log\left(\frac 1\delta\right) + (e - 1) \sum_{k = 1}^{m_T} 2^{-k} \frac{\Delta_0}{\sigma} \log\left(\frac{2^{k} \sigma \delta}{\Delta_0 h_k T}\right) (h_k - 1)\right)
    \end{align}
    Thus, let $h_k = 1$ for $k \leq 2 \log\left(\frac{\Delta_0 T}{\sigma \delta}\right) / \log(2)$ and let $h_k = 2^{\frac k 2}$ for larger $k$.  Then we see that with probability at least $1 - 2\delta$,
    \begin{equation}
        m_T \leq 2 \frac{\log\left(\frac T{2 \alpha + 1}\right)}{\log 2} + 2 \frac{\log\left(\frac{\Delta_0 T}{\sigma \delta}\right)}{\log 2} \leq 4 \frac{\log\left(\frac{\Delta_0 T}{\sigma \delta}\right)}{\log 2}
    \end{equation}
    and
    \begin{equation}
        \sum_{k = 1}^{m_T} 2^{-k} \frac{\Delta_0}{\sigma} \log\left(\frac{2^{k} \sigma \delta}{\Delta_0 h_k T}\right) (h_k - 1)\leq \sum_{j = 0}^\infty j \log(2) 2^{- \frac j2} \leq 4
    \end{equation}
    Thus, we have with probability at least $1 - 2\delta$,
    \begin{align}
        \reg_T \leq (2 \alpha + 1) \left(4 \frac{\log\left(\frac{\Delta_0 T}{\sigma \delta}\right)}{\log 2} + \log\left(\frac 1\delta\right)   + 8 \right)
    \end{align}
    as desired.  For the second statment, take $\delta = \frac 1T$.
\end{proof}
\ac{Add point about how this generalizes to the k-piece case.}
\ac{Does this argument work without robustifying large margin?}
