# Supplementary material for: Efficient and Near-Optimal Smoothed Online Learning for Generalized Linear Functions
Source: arXiv:2205.13056 source file (2022-05-25)
Supplement: Supplementary file 2 [file app_algs.tex]

%!TEX root = ../neurips_submission.tex

\section{Full Pseudocode}
