# Supplementary material for: Efficient and Near-Optimal Smoothed Online Learning for Generalized Linear Functions
Source: arXiv:2205.13056 source file (2022-05-25)
Supplement: Supplementary file 3 [file appendix_old.tex]

\section*{OLD STUFF}

In this note we extend some of the analysis of \cite{block2022smoothed} to more optimistic settings.  
\section{Halfspaces}
First, we consider the case of half spaces.  In particular, we consider the following setting.  Let $\cX \subset \rr^d$ be a compact set and let $\mu$ the normalized Lebesgue measure on $\cX$.  Let 
\begin{equation}
    \F = \left\{f(x) = \sign(w^T x + b) | w, b \in \rr^d \right\}
\end{equation}    
Suppose that at each time step $1 \leq t \leq T$, nature chooses some $p_t \in \Delta(\cX)$ that is $\sigma$-smooth with respect to $\mu$ and draws $x_t \sim p_t$.  The learner guesses $\yhat_t$ and nature reveals $y_t \in \{\pm 1\}$.  Letting $\ell$ denote indicator loss, we are concerned with
\begin{equation}
    \reg_T = \sum_{t = 1}^T \ell(\yhat_t, y_t) - \inf_{f \in \F} \sum_{t = 1}^T \ell(f(x_t), y_t)
\end{equation}
We first are concerned with the max-margin estimator in the realizable setting.  More precisely, suppose that $x_{1:t}, y_{1:t}$ are drawn and there exists some $f \in \F$ such that $f(x_s) = y_s$ for all $1 \leq s \leq t$.  Define the margin of the data set as
\begin{equation}
    \gamma_t(w, b) = \min_{x_s} y_s (w^T x_s + b)
\end{equation}
and let the max margin estimator be the interpolator maximizing this margin:
\begin{align}
    (w_t, b_t) = \argmax_{\substack{w, b \\ \norm{w} = 1 \\ \gamma_t(w, b) \geq 0}} \gamma(w, b) && f_t(x) = w_t^T x + b_t
\end{align}

We have the following result: \ac{Compare to Novikoff's margin based bound implied by control of the margin.}
\begin{proposition}
    Suppose that we are in the situation described above and suppose further that there is some $f \in \F$ such that $f(x_t) = y_t$ for all $1 \leq t \leq T$, i.e., $f_t$ is well-defined.  Then, with probability at least $1 - \delta$,
    \begin{equation}
        \reg_T \lesssim 3 \log\left(\frac{\diam \cX}{\sigma}\right) + 2 \cdot \sqrt[]{\log\left(\frac 1\delta\right)} + 2 \cdot \sqrt[]{T}
    \end{equation}  
    In particular,
    \begin{equation}
        \ee\left[\reg_T\right] \lesssim \log\left(\frac{T \diam \cX}{\sigma}\right) + \sqrt{ T}
    \end{equation}
\end{proposition}
\begin{proof}
    Fix a set of $0 < \epsilon_m < 1$ and let $t_0 = 0$.  For $m > 0$, let
    \begin{equation}
        t_m = \min\left\{t > t_{m-1} | \yhat_t \neq y_t\right\}
    \end{equation}
    Let $\Delta_t = 2 \gamma(w_t, b_t)$ be the size of the margin of the history and denote by $\Delta_m = \Delta_{t_m}$.  We claim that $\Delta_{m+1} \leq \frac{\Delta_m}{2}$.  To see this, note that at $t = t_m$, realizability implies that $\abs{w_{t-1}^T x_t + b_{t-1}} < \frac{\Delta_{m-1}}2$.  Define
    \begin{equation}
        \widetilde{f}_t = \sign\left(w_{t-1}^T x + b_{t-1}  - \frac{w_{t-1}^T x_t + b_{t-1} + \frac{\Delta_{t-1}}{2}}{2}\right)
    \end{equation}
    where, again, $\Delta_{t-1}$ is twice the margin of the history up to time $t-1$.  By the definition of margin, for $s < t$, we see that $\widetilde{f}_t(x_s) = y_s$ and has margin at most $\frac{\Delta_{t-1}}{2}$ by the fact that $\frac{\Delta_{t-1}}{2} - w_{t-1}^T x_t - b_{t-1}$ is nonnegative.  Thus we see that
    \begin{align}
        \frac{\Delta_t}{2} \leq y_t \left(w_{t-1}^T x_t + b_{t-1}  - \frac{w_{t-1}^T x_t + b_{t-1} + y_t\frac{\Delta_{t-1}}{2}}{2}\right) &= y_t \frac{w_{t-1} x_t + b_{t-1}}{2} + \frac{\Delta_{t-1}}{4} \leq \frac{\Delta_{t-1}}{4}
    \end{align}
    by the assumption of the mistake at $t = t_m$.  Thus we have $\Delta_{m} \leq \frac{\Delta_{m-1}}{2}$ as desired.  By induction,
    \begin{equation}
        \Delta_m \leq 2^{-m} \cdot \diam \cX  \label{eq:deltadecay}
    \end{equation}
    We now claim that there is some $c > 0$ such that with probability at least $1 - \delta$, for all $m \in \mathbb{N}$,
    \begin{equation}
        t_m \geq c m - \log\left(\frac 1\delta\right) + \sum_{k = 1}^m \log\left(\frac{\sigma}{\Delta_k}\right) \label{eq:mgrowth}
    \end{equation}
    To see this, note that $t_m = t$ only if $\abs{w_{t-1}^T x_t + b_{t-1}} < \Delta_m$.  By smoothness, this can only happen with probability $\frac{\Delta_t}{\sigma}$.  Let $\pi_m = \min\left(\frac{\Delta_m}\sigma, 1\right)$ and let $X_m$ be a random variable distributed geometrically with parameter $\pi_m$.  Then the preceding probability bound guarantees that $t_{m+1} - t_m$ is stochastically dominated by $X_m$.  Thus, for any $\lambda < - \log(1 - \pi_m)$,
    \begin{equation}
        \ee\left[e^{\lambda (t_{m+1} - t_m)}\right] \leq \ee\left[e^{\lambda X_m}\right] = \frac{\pi_m e^\lambda}{1 - (1 - \pi_m)e^\lambda}
    \end{equation}
    Thus if we let
    \begin{equation}
        B_m^\lambda = e^{\lambda t_m - m \lambda - \sum_{k = 1}^m \log \pi_k} \prod_{k = 1}^m \left(1 - (1 - \pi_k) e^\lambda\right) \label{eq:tsupermart}
    \end{equation}
    then for any $\lambda \leq 0$, $B_m^\lambda$ is a nonnegative supermartingale starting at $1$.  Thus setting $\lambda = -1$ and again applying Ville's inequality, we have that with probability at least $1 - \delta$, for all $m$,
    \begin{equation}
        t_m \geq m + \sum_{k = 1}^m \log\left(1 - (1 - \pi_k)e^{- 1}\right) + \sum_{k  = 1}^m \log\left(\frac{1}{\pi_k}\right) - \log\left(\frac 1\delta\right)
    \end{equation}
    We further note that
    \begin{align}
        \log\left(1 - (1 - \pi_k)e^{-1}\right) &\geq 1 - \frac{1}{1 - (1 - \pi_k)e^{-1}} = - \frac{(1 - \pi_k)e^{-1}}{1 - (1 - \pi_k)e^{-1}} \\
        &\geq - \frac{e^{-1}}{1 - e^{-1}}
    \end{align}
    Let
    \begin{equation}
        c = 1 - \frac{e^{-1}}{1 - e^{-1}} > 0
    \end{equation}
    Thus we have that with probability at least $1 - \delta$ that for all $m$,
    \begin{equation}
        t_m \geq c m - \log\left(\frac 1\delta\right) + \sum_{k = 1}^m \max\left(\log\left(\frac{\sigma}{\Delta_k}\right), 0\right)
    \end{equation}
    and \eqref{eq:mgrowth} follows immediately.

    Combining \eqref{eq:deltadecay} and \eqref{eq:mgrowth}, we have that with probability at least $1 - \delta / 2$, for all $m$,
    \begin{align}
        t_m &\geq c m - \log\left(\frac 1\delta\right) + \sum_{k = 1}^m \log\left(\frac{\sigma}{\Delta_k}\right) \\
        &\geq cm - \log\left(\frac 2\delta\right) - m \log\left(\frac{\diam \cX}{\sigma}\right) - \sum_{k = 1}^m\log\left(2^m\right) \\
        &\geq cm - \log\left(\frac 2\delta\right) - m \log\left(\frac{\diam \cX}{\sigma}\right) + \frac{\log 2}{2}m^2 \\
        &\geq \frac{\log 2}{2}m^2 - m \log\left(\frac{\diam \cX}{\sigma}\right) - \log\left(\frac 2\delta\right)
    \end{align}
    Thus if
    \begin{align}
        m \geq  3 \log\left(\frac{\diam \cX}{\sigma}\right) + 2 \cdot \sqrt[]{\log\left(\frac 1\delta\right)} + 2 \cdot \sqrt[]{T}
    \end{align}
    then with probability at least $1 - \delta$, $t_m > T$.  
\end{proof}
Note that this technique applies more generally in the realizable setting.  Let 
\begin{align}
    \F_t &= \left\{f \in \F | f(x_s) = y_s \text{ for all } s \leq t\right\} \\
    \cX_t &= \left\{x \in \cX | \text{ there exist } f, f' \in \F \text{ such that } f(x) \neq f(x')\right\}
\end{align}
If we are in the $\sigma$-smoothed online learning setting and we can guarantee for some $\epsilon, \epsilon' < 1$ that with probability at least $1 - \epsilon'$,
\begin{equation}
    \mu(\cX_{m+1}) \leq (1 - \epsilon) \mu(\cX_m)
\end{equation}
then the same argument applies.

We now show that the upper bound is tight asymptotically as $\sigma \downarrow 0$. \ac{Read over and fix in light of correction of above}
\begin{proposition}
    Suppose we are in the earlier setting.  Then there is a realizable adversary such that any classifier experiences
    \begin{equation}
        \ee\left[\reg_T\right] \gtrsim \log\left(\frac T\sigma\right)
    \end{equation}
\end{proposition}
\begin{proof}
    We construct the adversary as follows.  Fix $0 < \epsilon < 1$ and suppose that at each time $t$, the max margin classifier is given by $f_t(x) = w_t^T x + b_t$ with margin $\Delta_t$.  We let
    \begin{align}
        R_t = \left\{x \in \cX | (1 - \epsilon) \Delta_t \leq \abs{f_t(x)} \leq \Delta_t \right\}
    \end{align}
    We let the adversary select the distribution that picks uniformly from $R_t$ with probability $\min\left(\frac{\mu(R_t)}{\sigma}, 1\right)$ and with remaining probability selects $0$.  If $\abs{f_t(x_{t+1})} \geq \gamma$, then $y_t$ is determined by realizability.  Otherwise, let $y_t$ be an independent Rademacher random variable.

    Let $\pi_m = \min\left(\frac{\epsilon \Delta_m}{\sigma}, 1\right)$ with $\Delta_m$ the margin as above.  Letting $t_m$ be the $m^{th}$ time that $x_t \in R_t$, we see that $t_{m+1} - t_m$ is geometrically distributed with parameter $\pi_m$ and thus \eqref{eq:tsupermart} is a supermartingale for $\lambda < \min_{k \leq m }\left(- \log(1 - \pi_k)\right) = - \log(1 - \pi_m)$.  Note that by construction, $\Delta_{m+1} \geq (1 - \epsilon) \Delta_m$ and thus $\Delta_m \geq (1 - \epsilon)^m$.  Setting $\lambda = \pi_m \leq - \log(1 - \pi_m)$ and applying Ville's inequality with \eqref{eq:tsupermart}, we get that with probability at least $ 1- \delta$, for all $m$,
    \begin{align}
        t_m \leq m + \frac{\log\left(\frac{1}{\delta}\right)}{\pi_m} +\frac 1{\pi_m} \sum_{k = 1}^m \log\left(\frac{\pi_k}{1 - (1 - \pi_k)e^{\pi_k}}\right) 
    \end{align}
    We now note that
    \begin{align}
        \frac{1}{\pi_m} \log\left(\frac{\pi_k}{1 - (1 - \pi_k)e^{\pi_k}}\right)  &\leq \frac 1{\pi_m}\left(\frac{\pi_m}{1 - (1 - \pi_m)e^{\pi_m}} - 1 \right) \\
        &= \frac{e^{\pi_m} - 1}{\pi_m} \frac{1 - \pi_m}{1 - (1 - \pi_m)e^{\pi_m}} \\
        &\leq (e - 1) \frac{2}{\pi_m^2}
    \end{align}
    using monotonicity, the fact that $\pi_m \leq 1$ and the following computation:
    \begin{equation}
        1 - (1-x) e^x = 1 - (1-x) \sum_{k = 0}^\infty \frac{x^k}{k!} = \sum_{k =2}^\infty x^k \left(\frac{1}{(k-1)!} - \frac{1}{k!}\right) \geq \frac{x^2}{2}
    \end{equation}
    Now, using the fact that $\pi_m \geq \frac \epsilon \sigma (1 - \epsilon)^m$, we have
    \begin{align}
        t_m \leq m + \frac{\sigma}{\epsilon}(1 - \epsilon)^{-m} \log\left(\frac 1\delta\right) + 2 (e - 1)m\left(\frac{\epsilon}{\sigma}\right)^{-2} (1 - \epsilon)^{-2m} 
    \end{align}
    Setting $\epsilon = 1 - e^{-1}$, we see that there is some constant $c > 0$ such that with probability at least $1 - \delta$,
    \begin{align}
        t_m \leq c \max\left(\sigma e^{m} \log\left(\frac 1\delta\right), m \sigma^2 e^{2m}\right)
    \end{align}
    In particular, there is a universal constant $C$ such that if $m = C \log\left(\frac{T}{\sigma \log\left(\frac 1\delta\right)}\right)$, then with probability at least $1 - \delta$ we have $\reg_T \geq m$ because the probability of a mistake, given that $x_t \in R_t$ is $\frac 12$.  The result follows.
\end{proof}
Note that if we compare our upper and lower bounds as $\sigma \downarrow 0$, the ratio goes to a constant.
\ac{Adapt this argument to general $\mu$ not just Lebesgue.  Also to $k$-piece thresholds.  Move on to $k$-piece, degree $p$ polynomials.}

% \section{Better rate}
% Suppose we are in the realizable smoothed online learning setting, and let
% \begin{align}
%     \F_t &= \left\{f \in \F | f(x_s) = y_s \text{ for all } s \leq t\right\} \\
%     D_t &= \left\{x \in \cX | \text{ there exist } f, f' \in \F_t \text{ such that } f(x) \neq f'(x)\right\}
% \end{align}
% We have the following result:
% \begin{proposition}\label{prop:logarithmicrate}
%     Suppose we are in the above situation and let $\Delta_t$ such that for all $t$ we have  $\Delta_t \geq \mu(D_t)$.  Suppose that every time we make a mistake, $\Delta_t$ drops by a factor of $c$ for some $c < 1$.  Then, with probability at least $1 - \delta$,
%     \begin{align}
%         \reg_T \leq 4 \frac{\log\left(\frac{2T \Delta_0}{\sigma \delta}\right)}{\log\left(\frac 1c\right)} + \frac{e - 1}{1 - \sqrt[]{c}}
%     \end{align}
%     In particular,
%     \begin{equation}
%         \ee\left[\reg_T\right] \lesssim \frac{\log\left(\frac{T \Delta_0}{\sigma}\right)}{\log\left(\frac 1c\right)} + \frac{1}{1 - \sqrt[]{c}}
%     \end{equation}
% \end{proposition}
% \begin{proof}
%     Fix a set of positive integers $h_k$ for $k \in \mathbb{N}$.  Let $\tau_0 = 0$ and for all $m > 0$, let
%     \begin{equation}
%         \tau_m = \tau_{m-1} + \inf\left\{k > 0 \bigg| \sum_{t = \tau_{m-1} + (k-1)h_m}^{\tau_{m-1} + k h_m} \mathbb{I}[\yhat_t \neq y_t] > 0 \right\}
%     \end{equation}
%     Furthermore, let $T(m) = \sum_{k = 1}^{m} (\tau_k - \tau_{k-1}) h_k$ and
%     \begin{equation}
%         t_m = \inf\left\{t > T(m-1) | \yhat_t \neq y_t\right\}
%     \end{equation}
%     In words, we consider epochs of length $h_m$, whose length can change every time we make a mistake in an epoch.  We have $T(m)$ the time of the $m^{th}$ change of epoch and $\tau_m$ the number of epochs of length $h_m$ we have to go before we make a mistake; we also have $t_m$ is the time of the first mistake after the $m^{th}$ change of epoch size.  Let
%     \begin{equation}
%         A_m = \sum_{k = 1}^m \sum_{s = t_m + 1}^{T(m) - 1} \mathbb{I}[\yhat_s \neq y_s]
%     \end{equation}
%     be the number of mistakes in a given epoch other than the first mistake.  Let $\pi_m = \min\left(\frac{\Delta_m}{\sigma}, 1\right)$.  We first claim that with probability at least $1 - \delta$, for all $m$ it holds that:
%     \begin{equation}
%         A_m \leq \log\left(\frac 1\delta\right) + (e-1) \sum_{k = 1}^m \pi_k (h_k - 1) \label{eq:extramistakes}
%     \end{equation}
%     To see this, let
%     \begin{equation}
%         B_m^\lambda = \exp\left(\lambda A_m - \left(e^\lambda - 1\right)\sum_{k = 1}^m \pi_k h_k \right)
%     \end{equation}
%     We show that $B_m^\lambda$ is a supermartingale for all $\lambda > 0$.  To see this, we have
%     \begin{align}
%         \ee\left[B_m^\lambda | B_{m-1}^\lambda\right] = B_{m-1}^\lambda \ee\left[\exp\left(\lambda \sum_{s = t_m + 1}^{T(m) - 1} \mathbb{I}[\yhat_s \neq y_s] -\left(e^\lambda - 1\right) \pi_m (h_m - 1)\right) \bigg| B_{m-1}^\lambda \right] \leq B_{m-1}^\lambda
%     \end{align}
%     where the inequality follows because the conditional probability of a mistake for $t_m + 1 \leq T(m) - 1 \leq \pi_m$ by smoothness and realizability and $T(m) - 1 - (t_m + 1) \leq h_m - 1$ by construction.  Thus we may apply Ville's inequality and recover \eqref{eq:extramistakes}.

%     We now claim that with probability at least $1 - \delta$, it holds for all $m$ that
%     \begin{equation}
%         \tau_m - \tau_{m-1} \geq \max\left(1, \log\left(\frac{\delta}{\pi_m h_m T}\right)\right) \label{eq:tauseparation}
%     \end{equation}
%     To see this, let $X_m$ be a random variable distributed geometrically with parameter $\widetilde{\pi}_m = \min(h \pi_m, 1)$.  Then a union bound, realizability, and smoothness imply that $\tau_{m} - \tau_{m-1}$ is stochastically dominated by $X_m$.  Thus, for any $\lambda < - \log(1 - \pi_m)$,
%     \begin{equation}
%         \ee\left[e^{\lambda (\tau_{m} - \tau_{m-1})}\right] \leq \ee\left[e^{\lambda X_m}\right] = \frac{\widetilde{\pi_m} e^\lambda}{1 - (1 - \widetilde{\pi_m})e^\lambda}
%     \end{equation}
%     We further note that
%     \begin{align}
%         \log\left(1 - (1 - \widetilde{\pi}_m)e^{-1}\right) &\geq 1 - \frac{1}{1 - (1 - \widetilde{\pi}_m)e^{-1}} = - \frac{(1 - \widetilde{\pi}_m)e^{-1}}{1 - (1 - \widetilde{\pi}_m)e^{-1}} \\
%         &\geq - \frac{e^{-1}}{1 - e^{-1}}
%     \end{align}
%     Thus, setting $\lambda = -1$, we see that with probability at least $\frac{\delta}{T}$,
%     \begin{align}
%         \tau_m - \tau_{m-1} \geq  1 + \log\left(\frac 1 { \widetilde{\pi_m}}\right) -\log\left(\frac T\delta\right) - \frac{e^{-1}}{1 - e^{-1}} \geq \log\left(\frac{\delta}{h \pi_m T}\right)
%     \end{align}
%     a union bound, coupled with the fact that $\tau_m - \tau_{m-1} > 0$ by construction concludes the proof of \eqref{eq:tauseparation}.

%     Now we note that
%     \begin{equation}
%         T \geq T(m) = \sum_{k = 1}^m (\tau_k - \tau_{k-1}) h_k
%     \end{equation}
%     and, further, that if $m_T$ is the maximal $m$ such that the preceding display holds,
%     \begin{equation}
%         \reg_T \leq m_T + A_{m_T}
%     \end{equation}
%     Thus, combining \eqref{eq:extramistakes} and \eqref{eq:tauseparation}, along with the fact that $\pi_k \leq c^k \Delta_0 / \sigma$, with probability at least $1 - 2 \delta$, we have
%     \begin{align}
%         T &\geq \sum_{k = 1}^{m_T} \log\left(\frac{\sigma \delta}{c^k \Delta_0 h_k T}\right) h_k \label{eq:mTbound}\\
%         \reg_T &\leq m_T + \log\left(\frac 1\delta\right) + (e - 1) \sum_{k  =1}^m c^k \frac{\Delta_0}\sigma (h_k - 1) \label{eq:mTregbound}
%     \end{align}
%     Now, let $h_k = 1$ for $k \leq 2\log\left(\frac{ T \Delta_0}{\sigma \delta}\right) / \log\left(\frac 1c\right)$ and let $h_k = c^{- \frac k2}$ otherwise.  Then we see that if \eqref{eq:mTbound} and \eqref{eq:mTregbound} hold, then
%     \begin{equation}
%         m_T \leq 2\frac{\log T}{\log\left(\frac 1c\right)} + \frac{2\log\left(\frac{ T \Delta_0}{\sigma \delta}\right)}{\log\left(\frac 1c\right)} \leq - 4 \frac{\log\left(\frac{T \Delta_0}{\sigma \delta}\right)}{\log c}
%     \end{equation}
%     and
%     \begin{equation}
%         \sum_{k = 1}^m c^k \frac{\Delta_0}{\sigma}(h_k - 1) \leq \sum_{j = 0}^\infty c^{\frac j2} =  \frac{1}{1 - \sqrt{c}}
%     \end{equation}
%     Thus we see that with probability at least $1 - \delta$.
%     \begin{equation}
%         \reg_T \leq 4 \frac{\log\left(\frac{2T \Delta_0}{\sigma \delta}\right)}{\log\left(\frac 1c\right)} + \frac{e - 1}{1 - \sqrt[]{c}}
%     \end{equation}
%     which proves the first statement.  To get the bound in expectation, take $\delta = \frac 1T$.
% \end{proof}
% \ac{Put h constant in previous proof to recover lazy.}
